# Supplementary material for: P2FAAS: Toward Privacy-Preserving Fuzzing as a Service
Source: arXiv:1909.11164 source file (2019-09-24)
Supplement: Supplementary file 1 [file appendix.tex]

\appendix

\section{Appendix}

\subsection{List of Provisioned Audit Functions}
\label{s:app-design-audits}

\begin{table*}[t]
	\centering
	\scriptsize
	\definecolor{verygrey}{rgb}{0.9,0.9,0.9}
\begin{tabular}{clll}
	\toprule

  &
	\textbf{Item} &
	\textbf{Audit} &
	\textbf{Desc.} \\
	\midrule

  \parbox[c]{2mm}{\multirow{19}{*}{\rotatebox[origin=c]{90}{Packet metadata}}} & \\
  &
	\multirow{8}{*}{\cc{struct sk_buff}} &
	\cc{count_data()} &
	Accumulate the amount of data passed through. \\

  &
	&
	\cc{limit_bandwidth(bandwidth)} &
	Limit the rate of data under \cc{bandwidth}. \\

	&
  &
	\cc{count_packet()} &
	Accumulate the number of packets passed through. \\

  &
	&
	\cc{limit_rate(rate)} &
	Limit the rate of packets under \cc{rate}. \\

  &
	&
	\cc{limit_timestamp_freshness(within_time)} &
	Limit the timestamp of the packet under \cc{within_time} time from current time. \\

  &
	&
	\cc{count_ether_type(type)} &
	Count the number of packets with \cc{ether_type} matching \cc{type}. \\

  &
	&
	\cc{allow_ether_type(type)} &
	Allow packets with \cc{ether_type} matching \cc{type}. \\

  &
	&
	\cc{deny_ether_type(type)} &
	Deny packets with \cc{ether_type} matching \cc{type}. \\

	% \midrule
  \\
  &
	\multirow{6}{*}{Network header} &
	\cc{count_ip_single(ip)} &
	Count the number of packets from single address \cc{ip}. \\

  &
	&
	\cc{allow_ip_single(ip)} &
	Allow packets from single address \cc{ip}. \\

  &
	&
	\cc{deny_ip_single(ip)} &
	Deny packets from single address \cc{ip}. \\

  &
	&
	\cc{count_ip_range(ip1-ip2)} &
	Count the number of packets from addresses ranging between \cc{ip1} and \cc{ip2}. \\

	&
  &
	\cc{allow_ip_range(ip1-ip2)} &
	Allow packets from addresses ranging between \cc{ip1} and \cc{ip2}. \\

	&
  &
	\cc{count_ip_range(ip1-ip2)} &
	Deny packets from addresses ranging between \cc{ip1} and \cc{ip2}. \\

	% \midrule
  \\

  &
	\multirow{6}{*}{Transportation header} &
	\cc{count_port_single(port)} &
	Count the number of packets to single port number \cc{port}. \\

	&
  &
	\cc{allow_port_single(port)} &
	Allow packets to single port number \cc{port}. \\

	&
  &
	\cc{deny_port_single(port)} &
	Deny packets to single port number \cc{port}. \\

	&
  &
	\cc{count_port_range(port1-port2)} &
	Count the number of packets to port numbers ranging between \cc{port1} and \cc{port2}. \\

	&
  &
	\cc{allow_port_range(port1-port2)} &
	Allow packets to port numbers ranging between \cc{port1} and \cc{port2}. \\

	&
  &
	\cc{deny_port_range(port1-port2)} &
	Deny packets to port numbers ranging between \cc{port1} and \cc{port2}. \\

\midrule

\parbox[c]{2mm}{\multirow{12}{*}{\rotatebox[origin=c]{90}{Audit info}}} & \\
&
  \multirow{5}{*}{Presence} &
	\cc{allow_with_presence(label)} &
	Allow packets if label \cc{label(device)} is present in HAN. \\

	&
  &
	\cc{deny_with_presence(label)} &
	Deny packets if label \cc{label(device)} is present in HAN. \\

	&
  &
	\cc{record_presence()} &
	Record the most recent timestamps of both labels as presence history. \\

	&
  &
	\cc{allow_with_recent_presence(label, period)} &
	Allow packets if label \cc{label(device)} was present recently (within \cc{period}) in HAN. \\

	&
  &
	\cc{deny_with_recent_presence(label, period)} &
	Deny packets if label \cc{label(device)} was present recently (within \cc{period}) in HAN. \\

	% \midrule
  \\

  &
	\multirow{7}{*}{Time} &
	\cc{allow_hour_range(t1-t2)} &
	Allow packets if current hour of day is between \cc{h1} and \cc{h2}. \\

  &
	&
	\cc{deny_hour_range(t1-t2)} &
	deny packets if current hour of day is between \cc{h1} and \cc{h2}. \\

  &
	&
	\cc{allow_day(day)} &
	Allow packets if current day of week is \cc{day}. \\

  &
	&
	\cc{deny_day(day)} &
	Deny packets if current day of week is \cc{day}. \\

  &
	&
	\cc{allow_days([...day])} &
	Allow packets if current day of week is one of \cc{[...day]}. \\

  &
	&
	\cc{deny_days([...day])} &
	Deny packets if current day of week is one of \cc{[...day]}. \\

	&
  &
	\cc{count_down_hours(num)} &
	Start count down of \cc{num} hours. Allow packets during countdown and deny packets when countdown finishes. \\

	\bottomrule
\end{tabular}

	\caption{Provisioned audit functions in \sys}
	\label{tbl:audit-provisioned}
\end{table*}
